# Supplementary material for: Graphusion: A RAG Framework for Knowledge Graph Construction with a Global Perspective
Source: arXiv:2410.17600 source file (2025-02-03)
Supplement: Supplementary file 1 [file appendix_workshop.tex]

\section{Appendix}

\subsection{Reviewer 1}

The paper introduces Graphusion, a Retrieval-Augmented Generation (RAG) framework designed for the construction of scientific knowledge graphs (KGs) from free text with a global perspective. The framework addresses the limitations of existing methods that focus on local knowledge extraction by incorporating a knowledge fusion module. Graphusion consists of three main steps: seed entity extraction, candidate triplet extraction, and knowledge graph fusion. The framework has been evaluated on various tasks within the natural language processing (NLP) domain, including a new benchmark dataset called TutorQA, which contains 1,200 expert-verified question-answer pairs.
\textbf{Strengths:} 1. Graphusion offers a novel zero-shot KG construction framework that leverages large language models (LLMs) for global knowledge integration, which is a significant advancement over local extraction methods. 2.The paper demonstrates strong performance of Graphusion on entity extraction and relation recognition tasks, outperforming baselines and showcasing the effectiveness of the fusion step. 3.The focus on a global view of knowledge extraction is particularly important for scientific domains, where understanding complex, multi-layered relations is crucial.

\textbf{Questions:} \textbf{1. }The framework's reliance on multiple steps and the integration of LLMs may introduce complexity in implementation and computational costs, which could be a barrier for some users. Moreover, the article's lack of innovation is a pipeline-style prompt-aware approach that can suffer from error propagation problems, how can this be avoided? 
\textbf{2.} The article is not clear in its description of what is local KG and what is global KG? This is also not emphasised in the section on models and experiments. How the global KG fits into the model? 
\textbf{3.}How to ensure fairness when the model's assessment results are all manual. There is also a lack of expert information description, as well as a specific assessment process. 
\textbf{4.}While the human evaluation of constructed KGs provides valuable insights, the lack of a comprehensive automatic evaluation benchmark could limit the objectivity of the performance assessment.

\textbf{Ethics Review Flag:} No

\textbf{Scope: 4:} The work is relevant to the Web and to the track, and is of broad interest to the community

\textbf{Novelty: 4}

\textbf{Technical Quality: 4}

\textbf{Reviewer Confidence: 4: }The reviewer is certain that the evaluation is correct and very familiar with the relevant literature.

\subsection{Reviewer 2}
What is the problem being addressed? 
Cohesive global KGs from text using candidate triplets, topic modeling, and fusion from free text. There is both simple entity resolution and semantic (kind of) conflict resolution followed by new inference. LLM prompting is used to perform these tasks.
Why is it important?
It is an age-old problem, and using prompts to address it is interesting. The key is developing a prompt and testing the results.
What is related work? 
CauseKG: A Framework Enhancing Causal Inference With Implicit Knowledge Deduced From Knowledge Graphs Publisher: IEEE Cite This Hao Huang; Maria-Esther Vidal
Above is a paper on causal inference in KG. Some evaluation on the quality of KG triplets generated by LLM must be provided,
Do the results show that the problem is reasonably addressed?
The prompt does not explicitly say to use only the data provided and not to hallucinate. How did you test for the correctness of the results?
Step 1 uses existing techniques [17] and [11] and is limited by their performance. It is possible to miss some crucial entities. Why was LLM not used for entity extraction—using prompts? LLMs can also be used to remove irrelevant entities and correct errors. Has this been tried?
In Table 2, why did you not compare the entities extracted by GPT-4o with Graphusion? That would have been a more realistic comparison. You are comparing GRapgRAG with techniques [17] and [11], right?
There are issues in accuracy in Figure 3; how is this corrected? By humans?
Table 5 is not relevant to the evaluation as all three projects are equally good (from my perspective). What is Graphusion's specific contribution to changing the LLMs' response is unclear. Did you generate this by post-processing?
The paper says — “Lastly, with Graphusion constructed KG, the model provides a more comprehensive solution, elaborating on the enti- ties and introducing additional ones (highlighted in lavender) that come from the recovered graph, like dependency parsing and event extraction, while initially addressing the queried enti- ties.”
The paper does not detail how the above is done. Do you collate text from LLMs and get another text?
The appendix material does not provide the details.

\textbf{Questions:}
There are questions above which can be responded to.

\textbf{Ethics Review Flag:} No

\textbf{Scope: 3: }The work is somewhat relevant to the Web and to the track, and is of narrow interest to a sub-community

\textbf{Novelty: 3}

\textbf{Technical Quality: 3}

\textbf{Reviewer Confidence: 4}: The reviewer is certain that the evaluation is correct and very familiar with the relevant literature

\subsection{Reviewer 3}
This paper presents Graphusion, a knowledge graph construction (KGC) framework that provides a global view of the extracted knowledge. Specifically, the method consists of a three-step pipeline: seed entity generation, candidate triplet extraction, and knowledge graph fusion. In addition, the authors also construct an educational NLP QA benchmark TutorQA.
\textbf{Strengths:} The authors propose a novel KGC framework Graphusion that uses LLMs to automatically construct scientific Knowledge Graphs. The authors showcase Graphusion’s efficacy through both human evaluation and downstream QA performance. The authors conduct extensive case studies and analysis.
The authors propose an educational QA benchmark TutorQA, which consists of 6 sub-tasks that model real-world educational scenarios. This provides a valuable resource for evaluating KGC frameworks in an educational context.
\textbf{Weeknesses:}
This paper contains major formatting issues. There are no section numbers throughout the paper, making it hard for readers to determine the hierarchical relations between sections and sub-sections. There is also no section title for the “Introduction” section. These formatting issues make it very challenging for readers to understand the paper's organization, and raise questions of whether the authors strictly followed WWW’s template guidelines.
The presentation of the paper lacks sufficient clarity, making it challenging for readers to capture the author’s research motivation and contribution.
For instance, in the section titled “Graphusion: Zero-shot Knowledge Graph Construction”, the authors claim that their approach is designed to tackle three key challenges: (1) taking free text as input, (2) resolving conflicting relations, and (3) outputing a list of triplets. However, based on the author’s own problem definition of zero-shot KGC, it seems that both “(1) taking free text as input” and “(3) outputing a list of triplets” are naturally required by the KGC task, leaving “(2) resolving conflicting relations” as the only novel challenge addressed by Graphusion. This leads to confusion regarding the core contributions of the method.
Furthermore, the authors present a long section at the middle of the paper to evaluate LLMs conducting link prediction, which is irrelevant to either their proposed method or dataset, making readers questioning their contribution.
The paper’s research topic and methodology demonstrates limited relevance to the Web and the track.
In terms of the Web, this paper primarily focuses on the use of static offline data (e.g., downloaded research paper abstracts), without addressing how Graphusion interacts with or contributes to the Web.
In terms of the track, instead of focusing on retrieval-augmented AI (i.e. enhancing model performance with retrieved data) , Graphusion contributes more to the modeling of data (i.e. knowledge graph construction using retrieved data), which fits better into other tracks such as “Semantics and Knowledge”.

\textbf{Questions:}
What is GraphRAG’s “community aggregation” step? What is the concrete difference between your “knowledge fusion” step and GraphRAG’s “community aggregation” step, since both of them seem to be integrating multiple sub-graphs into one? How is your “knowledge fusion” step better than “community aggregation”?
How is the Link Prediction experiments section related to your proposed Graphusion method? For your research, why is it important to evaluate LLM conducting Link Prediction?

\textbf{Ethics Review Flag:} No

\textbf{Scope: 1:} The work is irrelevant to the Web

\textbf{Novelty: 3}

\textbf{Technical Quality: 2}

\textbf{Reviewer Confidence: 3}: The reviewer is confident but not certain that the evaluation is correct.

\subsection{Reviewer 4}

This paper introduces a zero-shot knowledge graph construction framework named Graphusion, aimed at automatically constructing scientific knowledge graphs from free text. The Graphusion framework consists of three core steps: entity extraction, candidate triple extraction, and fusion module design. Through these steps, Graphusion can integrate knowledge from a global perspective, addressing the issue that existing methods mainly focus on local knowledge extraction. Experimental results show that Graphusion achieved scores of 2.92 and 2.37 (out of 3) in entity extraction and relation recognition, respectively. Additionally, the paper introduces the TutorQA benchmark test, demonstrating Graphusion's potential in educational scenarios and significantly improving the accuracy of question-answering tasks.
Pros:
The paper proposes the Graphusion framework, a zero-shot knowledge graph construction method that can extract entities and relationships from free text and integrate global knowledge through a fusion module, solving the problem that existing methods primarily focus on local knowledge extraction.
The paper details the three core steps of Graphusion: entity extraction, candidate triple extraction, and fusion module design, with clear objectives and technical implementations for each step.
The paper validates the effectiveness of Graphusion through the TutorQA benchmark test, showcasing its potential in educational settings.
The experimental section is thorough, comparing different settings (such as using only the base model, adding extra data, etc.) and providing ablation study results, further proving the effectiveness of each component.
Cons:
The paper mentions that in some cases, adding extra data (such as LectureBankCD documents) can reduce performance, possibly due to the introduction of noise and overly long content. This part could be further explored to determine how to effectively filter and refine external data.
Although the paper demonstrates Graphusion's application in the NLP field, its generalizability needs to be verified in other domains.

\textbf{Questions:}
You mentioned that adding external data (such as LectureBankCD documents) sometimes reduces model performance. Could you provide more specific reasons for this phenomenon? Are there methods to more effectively screen and utilize this external data to avoid introducing noise?
How are entity merging, conflict resolution, and the discovery of new triples specifically implemented in the fusion module? Could you provide more technical details and experimental results to support the effectiveness of these functions?
The TutorQA benchmark test covers six tasks. What are the specific designs and evaluation criteria for each task? Could you provide some concrete examples to illustrate the practical applications of these tasks?

\textbf{Ethics Review Flag: No}

\textbf{Scope: 3:} The work is somewhat relevant to the Web and to the track, and is of narrow interest to a sub-community

\textbf{Novelty: 6}

\textbf{Technical Quality: 6}

\textbf{Reviewer Confidence: 3:} The reviewer is confident but not certain that the evaluation is correct.

\section{Improvements}

After carefully reviewing the feedback, we addressed most of the concerns raised by the reviewers. These include: clarifying the criteria for human evaluation (raised by R1 and R2) in the section \textbf{TutorQA}; comparing our approach with GraphRAG (raised by R4) in Table 2; and adding a discussion on generalizability (raised by R3 and R4) in the section \textbf{Extension on Japanese Medical Data}. Other clarifications are made in different sections, including how to understand global and local information, seed entity generation details of Graphusion, and technical questions about TutorQA.
